# Supplementary material for: A Variational Approach to Enhanced Sampling and Free Energy Calculations
Source: arXiv:1407.0477 ancillary file (2014-08-07)
Supplement: Supplementary file 1 [file SM_arXiv1407-0477v3_ValssonParrinello.pdf]

# Supplemental Material for 'A Variational Approach to Enhanced Sampling and Free Energy Calculations'

Omar Valsson[1,*] and Michele Parrinello[1,†]

[1]*Department of Chemistry and Applied Biosciences, ETH Zurich and Facoltà di Informatica, Instituto di Scienze Computationali, Università della Svizzera italiana, Via Giuseppe Buffi 13, CH-6900, Lugano, Switzerland.*

(Dated: August 5, 2014)

* omar.valsson@phys.chem.ethz.ch

† parrinello@phys.chem.ethz.ch

SM for arXiv:1407.0477v3

This Supplemental Material contains the following five sections:

I Additional Properties of the $\Omega[V]$ Functional

II Further Details on the Fourier Series Basis Set

III Obtaining Free Energy Surfaces by Reweighting

IV Computational Details

V Additional Results and Free Energy Surfaces

## I. ADDITIONAL PROPERTIES OF THE $\Omega[V]$ FUNCTIONAL

Here we consider some additional properties of the $\Omega[V]$ functional defined in Eq. 2 in the paper as

$$\Omega[V] = \frac{1}{\beta}\log\frac{\int d\mathbf{s}\, e^{-\beta[F(\mathbf{s})+V(\mathbf{s})]}}{\int d\mathbf{s}\, e^{-\beta F(\mathbf{s})}} + \int d\mathbf{s}\, p(\mathbf{s})V(\mathbf{s}) \tag{S1}$$

where $p(\mathbf{s})$ is an arbitrary probability distribution that is assumed to be normalized, $\int d\mathbf{s}\, p(\mathbf{s}) = 1$. The second term can thus be considered as an expectation value of $V(\mathbf{s})$ over the distribution $p(\mathbf{s})$.

### A. Invariance Under Addition of an Arbitrary Constant to $V(\mathrm{s})$

For any arbitrary constant $k$ that does not depend on s we have the following

$$\begin{aligned}\Omega[V+k] &= \frac{1}{\beta}\log\frac{\int d\mathbf{s}\, e^{-\beta[F(\mathbf{s})+V(\mathbf{s})+k]}}{\int d\mathbf{s}\, e^{-\beta F(\mathbf{s})}} + \int d\mathbf{s}\, p(\mathbf{s})\left[V(\mathbf{s})+k\right] \\ &= \frac{1}{\beta}\log\frac{\int d\mathbf{s}\, e^{-\beta[F(\mathbf{s})+V(\mathbf{s})]}}{\int d\mathbf{s}\, e^{-\beta F(\mathbf{s})}} + \underbrace{\frac{1}{\beta}\log e^{-\beta k}}_{=-k} + \int d\mathbf{s}\, p(\mathbf{s})V(\mathbf{s}) + k = \Omega[V],\end{aligned} \tag{S2}$$

where the constant $k$ can be taken out of both integrals. The functional is therefore invariant under the addition of an arbitrary constant constant $k$ to $V(\mathbf{s})$, $\Omega[V+k] = \Omega[V]$.

### B. Convexity of the Functional

The $\Omega[V]$ functional is convex, in other words, for any two potentials $V_1(\mathbf{s})$ and $V_2(\mathbf{s})$ the functional fulfils the inequality

$$\Omega\left[\frac{V_1+V_2}{2}\right] \leq \frac{1}{2}\Omega[V_1] + \frac{1}{2}\Omega[V_2]. \tag{S3}$$

In order to prove this we start by considering the following equation

$$\begin{aligned}\left(\int d\mathbf{s}\, e^{-\beta\left[F(\mathbf{s})+\frac{V_1(\mathbf{s})+V_2(\mathbf{s})}{2}\right]}\right)^2 &= \left(\int d\mathbf{s}\, e^{-\frac{\beta}{2}[F(\mathbf{s})+V_1(\mathbf{s})]}e^{-\frac{\beta}{2}[F(\mathbf{s})+V_2(\mathbf{s})]}\right)^2 \\ &\leq \int d\mathbf{s}\, e^{-\beta[F(\mathbf{s})+V_1(\mathbf{s})]} \cdot \int d\mathbf{s}\, e^{-\beta[F(\mathbf{s})+V_2(\mathbf{s})]},\end{aligned} \tag{S4}$$

SM for arXiv:1407.0477v3

where we have employed the Cauchy-Schwarz inequality in the last step. Dividing this equation by $\left(\int d\mathbf{s}\, e^{-\beta F(\mathbf{s})}\right)^2$ and taking the natural logarithm on both sides leads to

$$\frac{1}{\beta}\log\frac{\int d\mathbf{s}\, e^{-\beta\left[F(\mathbf{s})+\frac{V_1(\mathbf{s})+V_2(\mathbf{s})}{2}\right]}}{\int d\mathbf{s}\, e^{-\beta F(\mathbf{s})}} \le \frac{1}{2\beta}\log\frac{\int d\mathbf{s}\, e^{-\beta[F(\mathbf{s})+V_1(\mathbf{s})]}}{\int d\mathbf{s}\, e^{-\beta F(\mathbf{s})}} + \frac{1}{2\beta}\log\frac{\int d\mathbf{s}\, e^{-\beta[F(\mathbf{s})+V_2(\mathbf{s})]}}{\int d\mathbf{s}\, e^{-\beta F(\mathbf{s})}} \qquad \text{(S5)}$$

The left-hand side of this equation corresponds to the first term in $\Omega\left[\frac{V_1+V_2}{2}\right]$ while the two terms on the right-hand side correspond to the first term in $\frac{1}{2}\Omega[V_1]$ and $\frac{1}{2}\Omega[V_2]$, respectively. The second term in $\Omega[V]$ is linear in $V(\mathbf{s})$ so we have that

$$\int d\mathbf{s}\, p(\mathbf{s})\left[\frac{V_1(\mathbf{s})+V_2(\mathbf{s})}{2}\right] = \frac{1}{2}\int d\mathbf{s}\, p(\mathbf{s})V_1(\mathbf{s}) + \frac{1}{2}\int d\mathbf{s}\, p(\mathbf{s})V_2(\mathbf{s}). \qquad \text{(S6)}$$

Putting these two equations together results in

$$\begin{aligned}
&\frac{1}{\beta}\log\frac{\int d\mathbf{s}\, e^{-\beta\left[F(\mathbf{s})+\frac{V_1(\mathbf{s})+V_2(\mathbf{s})}{2}\right]}}{\int d\mathbf{s}\, e^{-\beta F(\mathbf{s})}} + \int d\mathbf{s}\, p(\mathbf{s})\left[\frac{V_1(\mathbf{s})+V_2(\mathbf{s})}{2}\right] \\
&\le \frac{1}{2}\left[\frac{1}{\beta}\log\frac{\int d\mathbf{s}\, e^{-\beta[F(\mathbf{s})+V_1(\mathbf{s})]}}{\int d\mathbf{s}\, e^{-\beta F(\mathbf{s})}} + \int d\mathbf{s}\, p(\mathbf{s})V_1(\mathbf{s})\right] \\
&+ \frac{1}{2}\left[\frac{1}{\beta}\log\frac{\int d\mathbf{s}\, e^{-\beta[F(\mathbf{s})+V_2(\mathbf{s})]}}{\int d\mathbf{s}\, e^{-\beta F(\mathbf{s})}} + \int d\mathbf{s}\, p(\mathbf{s})V_2(\mathbf{s})\right],
\end{aligned} \qquad \text{(S7)}$$

or

$$\Omega\left[\frac{V_1+V_2}{2}\right] \le \frac{1}{2}\Omega[V_1] + \frac{1}{2}\Omega[V_2], \qquad \text{(S8)}$$

which proves that $\Omega[V]$ is a convex functional.

### C. Stationary point of $\Omega[V]$

We obtain from calculus of variations that the potential $V(\mathbf{s})$ that renders $\Omega[V]$ stationary fulfils the following equation

$$0 = \frac{\partial\Omega[V]}{\partial V(\mathbf{s})} = -\frac{e^{-\beta[F(\mathbf{s})+V(\mathbf{s})]}}{\int d\mathbf{s}\, e^{-\beta[F(\mathbf{s})+V(\mathbf{s})]}} + p(\mathbf{s}), \qquad \text{(S9)}$$

leading to

$$\begin{aligned}
V(\mathbf{s}) &= -F(\mathbf{s}) - \frac{1}{\beta}\log p(\mathbf{s}) - \frac{1}{\beta}\log\int d\mathbf{s}\, e^{-\beta[F(\mathbf{s})+V(\mathbf{s})]} \\
&= -F(\mathbf{s}) - \frac{1}{\beta}\log p(\mathbf{s}) - \frac{1}{\beta}\log Z_V,
\end{aligned} \qquad \text{(S10)}$$

where $Z_V = \int d\mathbf{s}\, e^{-\beta[F(\mathbf{s})+V(\mathbf{s})]}$ is a constant that does not depend on $\mathbf{s}$ so the last term is a constant that normally can be ignored. The functional is convex so this stationary point corresponds to the global

SM for arXiv:1407.0477v3

minimum of $\Omega[V]$. Note that Eq. S9 is only fulfilled if the distribution $p(\mathbf{s})$ is assumed to normalized, $\int d\mathbf{s}\, p(\mathbf{s}) = 1$.

Putting Eq. S10 into $\Omega[V]$ gives that the value of $\Omega[V]$ at the global minimum is

$$\begin{aligned}\Omega[V] &= -\frac{1}{\beta}\log\int d\mathbf{s}\, e^{-\beta F(\mathbf{s})} - \int d\mathbf{s}\, p(\mathbf{s})\left[F(\mathbf{s}) + \frac{1}{\beta}\log p(\mathbf{s})\right] \\ &= -\frac{1}{\beta}\log Z - \langle F(\mathbf{s})\rangle_p - \frac{1}{\beta}\langle \log p(\mathbf{s})\rangle_p \end{aligned} \quad \text{(S11)}$$

### D. Estimating $\Omega[V]$ During the Optimization Process

For estimating $\Omega[V]$ during the optimization process it is better to rewrite it in the following manner

$$\begin{aligned}\Omega[V] &= \frac{1}{\beta}\log\frac{\int d\mathbf{s}\, e^{-\beta[F(\mathbf{s})+V(\mathbf{s})]}}{\int d\mathbf{s}\, e^{-\beta[F(\mathbf{s})+V(\mathbf{s})]}e^{\beta V(\mathbf{s})}} + \int d\mathbf{s}\, p(\mathbf{s})V(\mathbf{s}) \\ &= \frac{1}{\beta}\log\frac{1}{\left\langle e^{\beta V(\mathbf{s})}\right\rangle_V} + \langle V(\mathbf{s})\rangle_p \\ &= -\frac{1}{\beta}\log\left\langle e^{\beta V(\mathbf{s})}\right\rangle_V + \langle V(\mathbf{s})\rangle_p\,. \end{aligned} \quad \text{(S12)}$$

where we see that the first term is the expectation value of $e^{\beta V(\mathbf{s})}$ in a biased simulation with the potential $V(\mathbf{s})$. The $\langle V(\mathbf{s})\rangle_p$ term can in most cases be calculated analytically or numerically on a grid.

During the optimization process the sampling time for each iteration is generally too short to obtain a good estimate of $\left\langle e^{\beta V(\mathbf{s})}\right\rangle_V$. Instead we can estimate it as a running average from the start of the simulation. Another option is to estimate it as an exponential decaying average with some chosen decay time $\tau_D$ by using the equation $\bar{a}(t) = \frac{1}{\tau_D}\int_0^t dt'\, a(t')\cdot e^{-(t-t')/\tau_D}$ [1].

These averages are of course not correct during the initial part of the optimization when the bias potential is changing the most and adjusting to the free energy surface. Once the optimization process has reached convergence the bias potential will be in a quasi-stationary state and both averaging choices should yield a constant value of $\left\langle e^{\beta V(\mathbf{s})}\right\rangle_V$. We tried both options here and observed that either using a running average from the start or exponential decaying average with a decay time of of around $\tau_D \sim 100 - 1000$ ps gave similar indications of the convergence of the optimization process.

### E. The Probability Distribution $p(\mathbf{s})$

As discussed in the paper, the probability distribution $p(\mathbf{s})$ in $\Omega[V]$ determines the sampling of $\mathbf{s}$ when the bias potential $V(\mathbf{s})$ has converged. In the case of CVs defined in a compact space of volume $\Omega_{\mathbf{s}}$ the natural choice is to take a uniform distribution $p(\mathbf{s}) = \frac{1}{\Omega_{\mathbf{s}}}$. This results in a uniform sampling of all values in the CV

SM for arXiv:1407.0477v3

space and a direct relation between the bias potential and the free energy surface, $V(\mathbf{s}) = -F(\mathbf{s}) + \text{const}$.

For the case of unbounded CVs, $p(\mathbf{s})$ can be selected to limit the sampling to a specfic range of $\mathbf{s}$. This can for example be achived by selecting $p(\mathbf{s})$ to be a Gaussian distribution with a certain predefined mean and covariance matrix. Even for bound CVs it can be useful to take $p(\mathbf{s})$ different from a uniform distribution. This can for example be employed to localize the sampling to certain subspace in the CV space by selecting $p(\mathbf{s})$ to be a Gaussian distribution, or a Von Mises distribution in the case of periodic CVs. An example of the latter will be presented below in Section V C.

SM for arXiv:1407.0477v3

## II. FURTHER DETAILS ON THE FOURIER SERIES BASIS SET

In all examples in the paper we consider angular CVs that are periodic in the domain $[-\pi, \pi]$ and expand the bias potential in a Fourier series

$$V(\mathbf{s}) = \sum_{\mathbf{k}} \alpha_{\mathbf{k}} e^{i\mathbf{k}\mathbf{s}} = \sum_{k_1,k_2,\ldots,k_d} \alpha_{k_1,k_2,\ldots,k_d} \cdot e^{ik_1 s_1} \cdot e^{ik_2 s_2} \cdots e^{ik_d s_d} \tag{S13}$$

In practise we consider real expansion coefficients and take sine and cosine as our basis functions but use the complex form of the Fourier series here as it allows for more compact notation.

The integers $k_1, k_2, \ldots, k_d$ go from $-M$ to $M$ where $M$ is the highest term used in the Fourier series for each CV. We have here assumed that all CVs use the same number of basis functions but this is not necessary. The number of one-dimensional basis functions per CV is thus $(2 \cdot M + 1)$ and the total number of basis functions in the expansion of $V(\mathbf{s})$ is $(2 \cdot M + 1)^d - 1$ where we do not count the constant term that can be dropped from the expansion as discussed in the main paper.

It easy to see that apart from the constant term ($\mathbf{k} = \mathbf{0}$) that we ignore all the expectation values over the uniform distribution $p(\mathbf{s}) = \frac{1}{(2\pi)^d}$ are zero, $\left\langle e^{i\mathbf{k}\mathbf{s}} \right\rangle_p = \delta_{\mathbf{k},\mathbf{0}}$. This means that $\langle V(\mathbf{s}) \rangle_p = 0$ for all $V(\mathbf{s})$ which fixes the zero of $V(\mathbf{s})$ during minimization and allows us to judge convergence of the bias potential without any need to align the different potentials.

All other distributions $p(\mathbf{s})$ considered here (Gaussian and Von Mises distributions) are simplified by writing them as products of one-dimensional distributions which amount to ignoring the covariance between the CVs in $p(\mathbf{s})$. In this case the expectation values $\left\langle e^{i\mathbf{k}\mathbf{s}} \right\rangle_p$ become product of one-dimensional integrals that are easily computed numerically on a grid at the start of the simulation.

The Fourier expansion in Eq. S13 can be extended to CVs defined in different domains by making the substitution $k_i \rightarrow \frac{2\pi k_i}{L_i}$ where $L_i = s_{i,\text{max}} - s_{i,\text{min}}$ and $[s_{i,\text{min}}, s_{i,\text{max}}]$ is the domain of the CV $s_i$. In this case the uniform distribution is given by $p(\mathbf{s}) = \frac{1}{\prod_i L_i}$.

The Fourier expansion of $V(\mathbf{s})$ can also be used for general non-periodic CVs. The results at the boundaries of $V(\mathbf{s})$ will not be correct due to the enforced periodicity of the Fourier series but this can be solved by taking the domains $[s_{i,\text{min}}, s_{i,\text{max}}]$ of the CVs to be larger than the range of CV values one is interested in. Furthermore, the convergence of the optimization process is probably improved by not using an uniform $p(\mathbf{s})$ but rather a suitable $p(\mathbf{s})$ that localizes the sampling and avoids unnecessary sampling at the edges of $V(\mathbf{s})$. We show an example of this below in Section V D.

SM for arXiv:1407.0477v3

## III. OBTAINING FREE ENERGY SURFACES BY REWEIGHTING

The standard umbrella sampling relation between the unbiased distribution $P(\mathbf{R})$ and the biased distribution $P_V(\mathbf{R})$ where the bias potential $V(\mathbf{s}(\mathbf{R}))$ is acting on the system is given by

$$P(\mathbf{R}) \propto e^{\beta V(\mathbf{s}(\mathbf{R}))} P_V(\mathbf{R}). \tag{S14}$$

For the biased CVs $\mathbf{s}$ this results in

$$P(\mathbf{s}) = \int d\mathbf{R}\, \delta(\mathbf{s} - \mathbf{s}(\mathbf{R})) P(\mathbf{R}) \propto e^{\beta V(\mathbf{s})} P_V(\mathbf{s}). \tag{S15}$$

where $P_V(\mathbf{s}) = \int d\mathbf{R}\, \delta(\mathbf{s} - \mathbf{s}(\mathbf{R})) P_V(\mathbf{R})$ is the biased distribution for $\mathbf{s}$. The reweighted free energy surface is then apart from an unimportant constant given by

$$F(\mathbf{s}) = -\frac{1}{\beta} \log P_V(\mathbf{s}) - V(\mathbf{s}). \tag{S16}$$

This equation can be used to obtain $F(\mathbf{s})$ if the functional form for the bias potential $V(\mathbf{s})$ does not have the variational flexibility to fully describe the free energy surface. The biased distribution $P_V(\mathbf{s})$ is then estimated from the biased simulation, for example by a histogram or a kernel density estimation. Similar procedure has been used with good succes for metadynamics with adaptive Gaussians [1].

For some other set of CVs $\mathbf{s}'$, which might for example include a subset of the CVs $\mathbf{s}$, Eq. S14 results in

$$P(\mathbf{s}') \propto \int d\mathbf{R}\, \delta(\mathbf{s}' - \mathbf{s}'(\mathbf{R})) e^{\beta V(\mathbf{s}(\mathbf{R}))} P_V(\mathbf{R}). \tag{S17}$$

The unbiased distribution $P(\mathbf{s}')$ is estimated by a histogram or kernel density estimation where each point $\mathbf{s}'(\mathbf{R})$ is weighted by $e^{\beta V(\mathbf{s}(\mathbf{R}))}$. The reweighted free energy surface for $\mathbf{s}'$ is then obtained as $F(\mathbf{s}') = -\frac{1}{\beta} \log P(\mathbf{s}')$.

Although these equations assume a static bias potential the reweighting can also be done on the fly during the optimization process if the bias potential $V(\mathbf{s}(\mathbf{R}))$ quickly converges to a quasi-stationary state. All the reweighted free energy surfaces shown here are obtained with such on the fly reweighting and we do not observe any problems with this procedure.

SM for arXiv:1407.0477v3

## IV. COMPUTATIONAL DETAILS

### A. Model Systems

Three different benchmark systems are employed in the paper: 1) Alanine dipeptide (Ace-Ala-Nme) in vacuum. 2) Alanine dipeptide (Ace-Ala-Nme) solvated in a bath of 1200 water molecules. 3) $Ala_3$ (Ace-$Ala_3$-Nme) peptide in vacuum. In Fig. S1 we indicate the backbone dihedral angles used to describe the free energy surfaces of the alanine dipeptide and the $Ala_3$ peptide.

All systems are described by the Amber99-SB [2] force field and the TIP3P [3] water model is used for the solvent simulations.

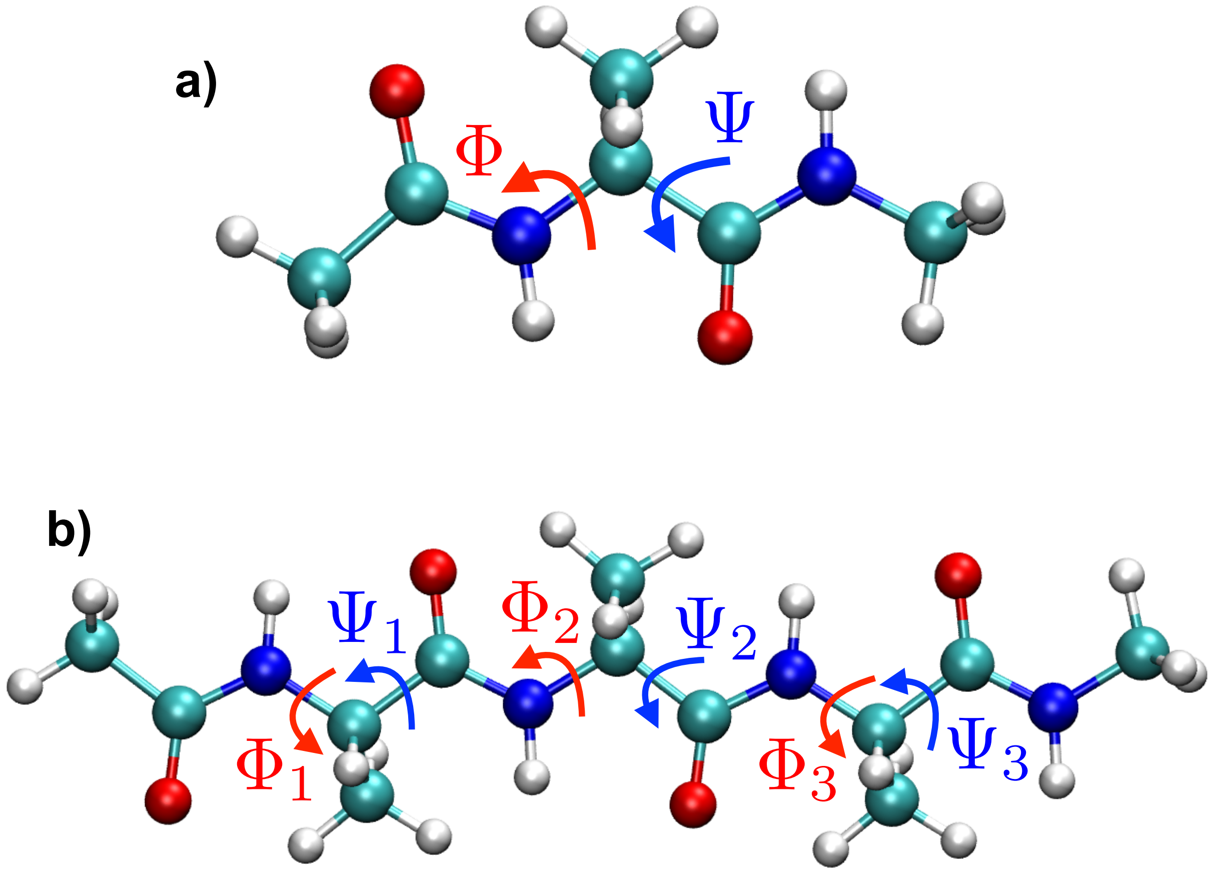


FIG. S1. The model systems employed in the paper along with the backbone dihedral angles used to describe their free energy surfaces. **a)** Alanine dipeptide (Ace-Ala-Nme) **b)** $Ala_3$ (Ace-$Ala_3$-Nme) peptide

SM for arXiv:1407.0477v3

### B. Molecular Dynamics Parameters

All molecular dynamics simulations for the alanine dipeptide and $Ala_3$ peptide are performed with the Gromacs 4.5.5 [4] MD code, patched with a private development version of the PLUMED 2 [5] enhanced sampling plug-in. We constrain bonds involving hydrogens using the LINCS [6] algorithm and employ a time-step of 0.002 fs in all simulations. The temperature is keep constant at 300K using the velocity rescaling thermostat [7] (relaxation time of 0.1 fs and 0.01 fs for the vacuum and solvent simulations, respectively).

We employ no periodic boundary conditions in the vacuum simulations and employ no cut-offs for the electrostatic and non-bonded Van der Waals interactions.

The simulations for the solvated alanine dipeptide are performed in the NVT ensemble using a periodic cubic box of side length 3.322 nm that included 1200 TIP3P water molecules. The long-range electrostatic interactions are handled using the Particle-Mesh Ewald [8] method with a real space cutoff of 1.2 nm. We employ a cutoff of 1.2 nm for the non-bonded Van der Waals interactions.

### C. Parameters for the Variational Approach

We employ a sampling time of 1.0 ps (500 steps) for each iteration in the optimization process in all calculations with the variational approach for the alanine dipeptide and the $Ala_3$ peptide.

The bias potential is always expanded in a Fourier series as described in Section II. For alanine dipeptide the number of basis functions used to expand the bias potential are indicated in the results. For $Ala_3$ we used 7 one-dimensional basis functions per CV which resulted in a total of 342 basis functions in the Fourier expansion of $V(\Phi_1, \Phi_2, \Phi_3)$. For alanine dipeptide (vacuum and solvent) we always use a step size of $\mu = 1.0$ kJ/mol and for $Ala_3$ we use a step size of $\mu = 0.02$ kJ/mol.

All results for the alanine dipeptide in vacuum and solvent are obtained after 10 ns and 20 ns, respectively, of simulations time, while the results for the $Ala_3$ peptide are obtained after 100 ns of simulation time. These simulations times were found well sufficient to reach convergence of the bias potential for all cases. This was also confirmed by running the simulations for longer times.

### D. Free Energy Surfaces for $Ala_3$

The projected two-dimensional free energy surfaces for the $Ala_3$ peptide shown in the paper in Fig 2**a)** and in Fig. S8**a)** below are obtained from the three-dimensional free energy surface $F(\Phi_1, \Phi_2, \Phi_3)$ by

SM for arXiv:1407.0477v3

integrating over one of the CVs. For example, the free energy surface $F(\Phi_1, \Phi_2)$ is obtained by integrating over $\Phi_3$

$$F(\Phi_1, \Phi_2) = -\frac{1}{\beta} \log \int d\Phi_3 \, e^{-\beta F(\Phi_1, \Phi_2, \Phi_3)}, \tag{S18}$$

so forth for other permutions of the CVs.

The reweighted free energy surfaces for $Ala_3$ shown in Fig 2**b)** in the paper and Figs. S8**b)** and S9**a)** below are obtained according to Eq. S17 above. For this we employ kernel density estimation where we sample values every 0.25 ps from the complete trajectory of the optimzation process (0-100 ns) and use Gaussian kernels with a bandwidth of 0.05 rad for all CVs.

### E. Well-Tempered Metadynamics for Alanine Dipeptide

The reference free energy surfaces for alanine dipeptide in vacuum and solvent are obtained from well-tempered metadynamics simulations using $\Phi$ and $\Psi$ as CVs. In these simulations, we employ a bias factor of 5, an initial Gaussian height of 1.2 kJ/mol, a Gaussian width of 0.2 rad for both $\Phi$ and $\Psi$, and deposit Gaussians every 1.0 ps (500 steps). The well-tempered metadynamics simulations are run for 100 ns for the vacuum system and for 200 ns for the solvated system.

### F. Parallel Tempering Simulations for $Ala_3$ in Vacuum

The reference free energy surfaces for the $Ala_3$ peptide in vacuum are obtained from parallel tempering simulation. We employ 8 replicas with temperatures distributed according to a geometrical distribution in the range 300 K to 1000 K. The simulation time for each replica was 500 ns, resulting in an aggregated simulation time of 4 $\mu$s. Exchanges between neighbouring replicas are attempted every 5 ps, resulting in average exchange acceptance of around 35% for all the replicas.

The free energy surfaces shown in Fig 2**c)** in the paper and Figs. S8**c)** and S9**b)** below are obtained by estimating the probability distributions of the CVs. This was done using kernel density estimation where we sample values every 0.25 ps from the whole 500 ns trajectory and use Gaussian kernels with a bandwidth of 0.05 rad for all CVs. Only the 300K replica is used for this analysis.

### G. Two-Dimensional Lennard-Jones Cluster

The computational details for the two-dimensional, seven-particle, Lennard-Jones cluster considered in Section V D are as follows. Note that we use reduced Lennard-Jones units for all parameters. The molecular

SM for arXiv:1407.0477v3

dynamics simulations are performed using the SimpleMD code in PLUMED 2 where the timestep is taken as 0.002 and the temperature is kept fixed at $T = 0.2$ using a Langevin thermostat [9] (friction constant 1.0). As in Ref. [10], we employ harmonic walls (force constants of 1000) at values of 0.4 and 1.2 for $\mu_2^2$ and -0.3 for $\mu_3^3$.

The coordination numbers are computed as $c_i = \sum_{i \neq j} \left[1 - \left(\frac{r_{ij}}{1.5}\right)^8\right] / \left[1 - \left(\frac{r_{ij}}{1.5}\right)^{16}\right]$ where $r_{ij}$ is the distance between particles $i$ and $j$. The CVs, corresponding to the second and third moments, $\mu_2^2$ and $\mu_3^3$, respectively, of the distribution of coordination numbers $c_i$ are defined as $\mu_2^2 = \frac{1}{N} \sum_{i=1}^{N} (c_i - \langle c \rangle)^2$ and $\mu_3^3 = \frac{1}{N} \sum_{i=1}^{N} (c_i - \langle c \rangle)^3$.

We take the domains of the CVs in the Fourier expansion for $V(\mu_2^2, \mu_3^3)$ as $[0.2, 1.4]$ for $\mu_2^2$ and $[-0.6, 1.6]$ for $\mu_3^3$. We employ 21 basis functions per CV for a total of 440 basis functions in the expansion of $V(\mu_2^2, \mu_3^3)$. We localize the sampling by taking $p(\mu_2^2, \mu_3^3)$ to be a two-dimensional Gaussian with mean at $\mu_2^2 = 0.8$, $\mu_3^3 = 0.5$ and standard deviation of 0.2 for $\mu_2^2$ and 0.4 for $\mu_3^3$. In the variational calculations the averages for each iteration are sampled over a time of 1.0 (500 steps) and we use a step size of $\mu = 0.001$. The simulation with the variational approach is run for $2 \cdot 10^5$ time units ($1.0 \cdot 10^8$ steps).

We also perform well-tempered metadynamics simulations to generate reference results. There we use a bias factor of 10, an initial Gaussian height of 0.02, Gaussian width of 0.02 for both CVs, and deposit Gaussian every 500 steps. The well-tempered metadynamics simulations is run for $9 \cdot 10^5$ time units ($4.5 \cdot 10^8$ steps).

SM for arXiv:1407.0477v3

## V. ADDITIONAL RESULTS AND FREE ENERGY SURFACES

### A. Free Energy Surfaces for Alanine Dipeptide in Vacuum and Water

We show in Fig. S2 free energy surfaces $F(\Phi, \Psi)$ for alanine dipeptide in vacuum obtained with the variational approach using both $\Phi$ and $\Psi$ as CVs and a different number of basis functions in the expansion of $V(\Phi, \Psi)$. In all the variational calculations the bias potential is well converged within 10 ns of simulation time. We can clearly observe that the variational results are in excellent agreement with reference metadynamics results shown in Fig. S2**f)**. From Fig. S2**a)** can we observe that even a minimal basis set of only 7 one-dimensional basis functions per CV, resulting in a total of 48 basis functions in the expansion of $V(\Phi, \Psi)$, gives a rather good representation of the free energy surface.

We also consider alanine dipeptide in solvent bath of 1200 water molecules and perform the same calculations using $\Phi$ and $\Psi$ as CVs and show the free energy surfaces obtained with the variational approach in Fig. S3. In all the variational calculations the bias potential is well converged within 20 ns of simulation time. Again we see that the variational results are in excellent agreement with reference metadynamics results shown in Fig. S3**f)**.

We can observe in Fig. S3**a)** that with the minimal basis set of 7 basis functions per CV do we obtain all the main features of the free energy surface. However, this minimal basis set is slightly lacking in variational flexibility to fully describe the finer features of the free energy basin in the top left corner of free energy surface. This can be corrected by performing on the fly reweighting of free energy surface using Eq. S16 above

$$F(\Phi, \Psi) = -\frac{1}{\beta} \log P_V(\Phi, \Psi) - V(\Phi, \Psi). \tag{S19}$$

In Fig. S4 we show the results of such reweighting where the biased distribution $P_V(\Phi, \Psi)$ was estimated by performing a kernel density estimation during the optimization process (which was run for 20 ns). We can observe in Fig. S4**b)** that the reweighted free energy surface is in very good agreement with the reference results.

SM for arXiv:1407.0477v3

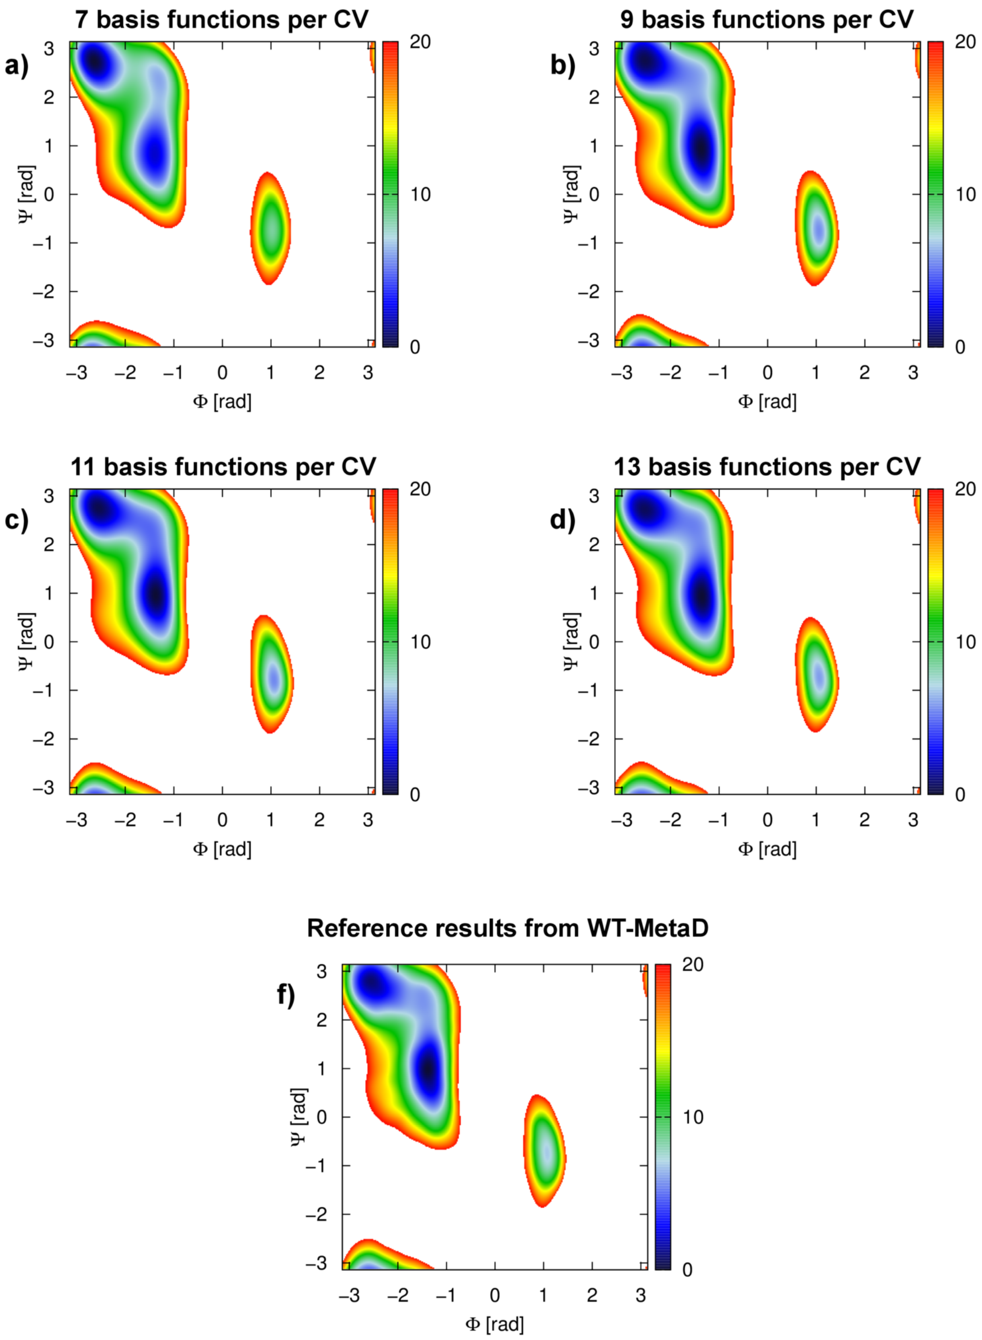


FIG. S2. FES $F(\Phi, \Psi)$ for alanine dipeptide in vacuum at 300 K obtained with the variational approach using both $\Phi$ and $\Psi$ as CVs.

Different number of basis functions are used in the expansion of $V(\Phi, \Psi)$ (see Section II): **a)** 7 per CV (total 48); **b)** 9 per CV (total 80); **c)** 11 per CV (total 120); **d)** 13 per CV (total 168). In panel **f)** we show for comparison reference results from a 100 ns well-tempered metadynamics simulation.

The color scale of the FES is given in units of kJ/mol. All FES have their minimum value set to zero and are cut such that regions higher than 8 $k_{\mathrm{B}}T$ ($\approx$ 20 kJ/mol) are not shown. The variational results are obtained after 10 ns of simulation time.

SM for arXiv:1407.0477v3

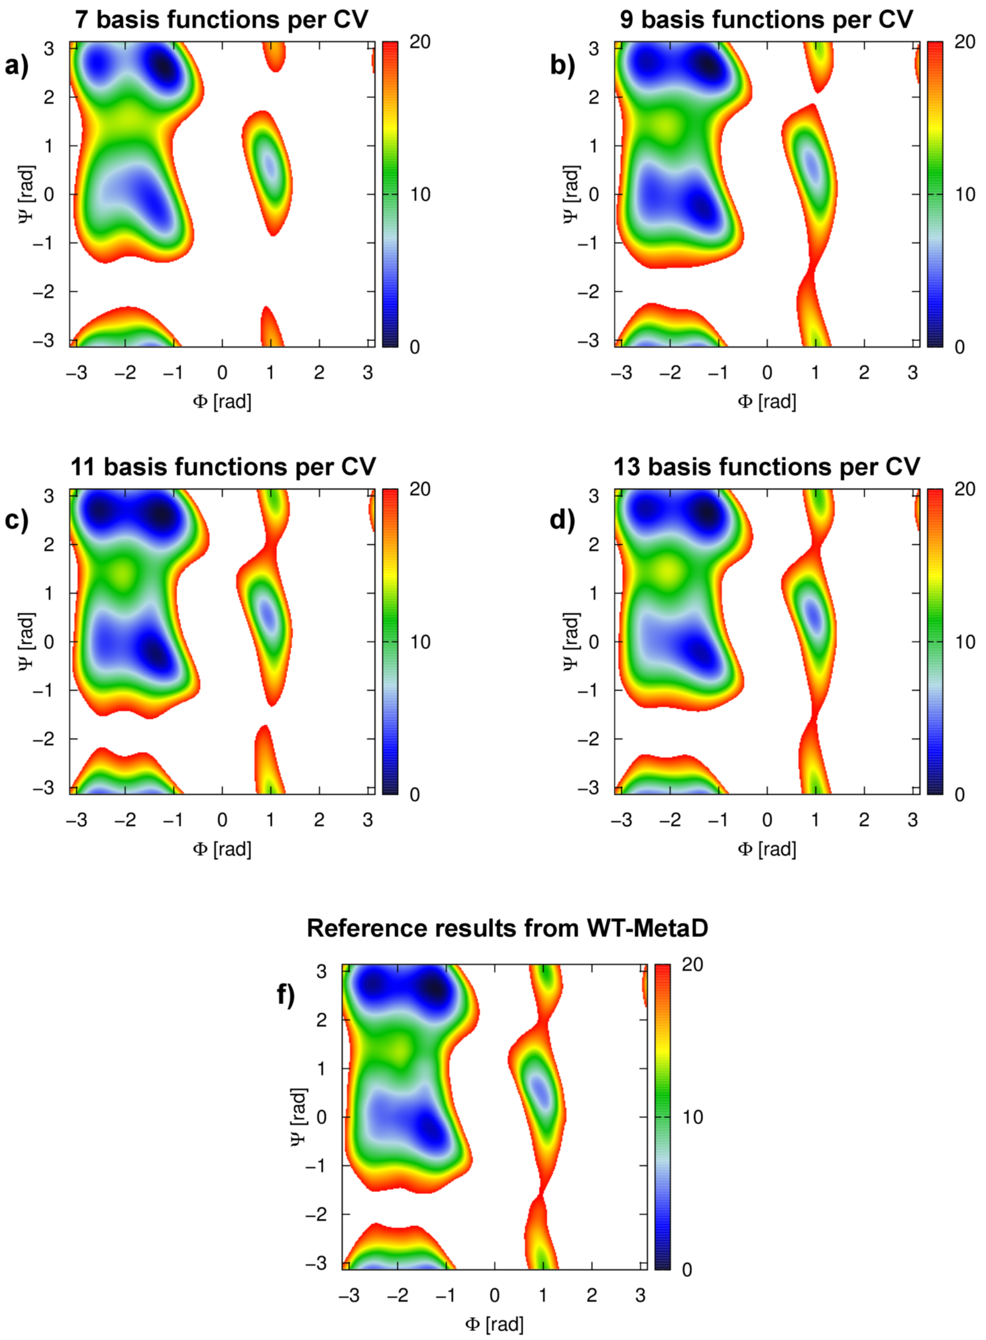


FIG. S3. FES $F(\Phi, \Psi)$ for alanine dipeptide in water (1200 TIP3P waters molecules) at 300 K obtained with the variational approach using both $\Phi$ and $\Psi$ as CVs.

Different number of basis functions are used in the expansion of $V(\Phi, \Psi)$ (see Section II): **a)** 7 per CV (total 48); **b)** 9 per CV (total 80); **c)** 11 per CV (total 120); **d)** 13 per CV (total 168). In panel **f)** we show for comparison reference results from a 200 ns well-tempered metadynamics simulation.

The color scale of the FES is given in units of kJ/mol. All FES have their minimum value set to zero and are cut such that regions higher than 8 $k_{\mathrm{B}}T$ ($\approx$ 20 kJ/mol) are not shown. The variational results are obtained after 20 ns of simulation time.

SM for arXiv:1407.0477v3

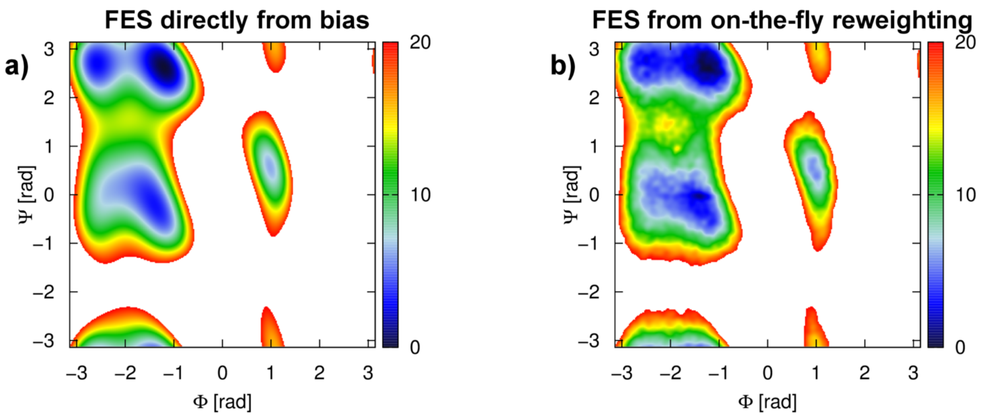


FIG. S4. The FES $F(\Phi,\Psi)$ for alanine dipeptide in water (1200 TIP3P waters) at 300 K obtained with the variational approach using both $\Phi$ and $\Psi$ as CVs and minimal basis set of 7 basis functions per CV.

**a)** The FES $F(\Phi,\Psi)$ obtained directly from the bias potential.

**b)** The FES $F(\Phi,\Psi)$ corrected for the lack of variational flexibility in the bias potential by using the equation $F(\Phi,\Psi) = -\frac{1}{\beta}\log P_V(\Phi,\Psi) - V(\Phi,\Psi)$ (Eq. S16 above). The biased distribution $P_V(\Phi,\Psi)$ is estimated by a kernel density estimation (Gaussian kernels with bandwidth of 0.05 rad for both CVs) during the optimization process (values sampled every 0.25 ps from the 20 ns simulation).

The color scale of the FES is given in units of kJ/mol. All FES have their minimum value set to zero and are cut such that regions higher than 8 $k_\mathrm{B}T$ ($\approx$ 20 kJ/mol) are not shown.

SM for arXiv:1407.0477v3

## B. Missing Slow Degree-of-Freedom

Like in metadynamics, a poor choice of the CVs, resulting in a missing slow degree of freedom, will manifest itself in a hysteresis behaviour during the optimization process of the variational approach. In order to show an example of this, we consider alanine dipeptide in vacuum where only $\Phi$ is a slow degree-of-freedom while $\Psi$ can be considered as a fast degree-of-freedom. Therefore, it is only needed to bias $\Phi$ in order to drive transistions between two basins and obtain a proper sampling of the phase space of the system. If we only employ $\Phi$ as a CV for the variational approach, the optimization process smoothly converges to correct results as shown in Fig. 1 in the main paper and we obtain a diffusive sampling of $\Phi$ as shown in Fig. S5**a)** here. However, as shown in Fig. S5**b)**, we observe a clear hysteresis behaviour in $\Psi$ if we only bias $\Psi$ and are missing the slow degree-of-freedom $\Phi$ from the CV set.

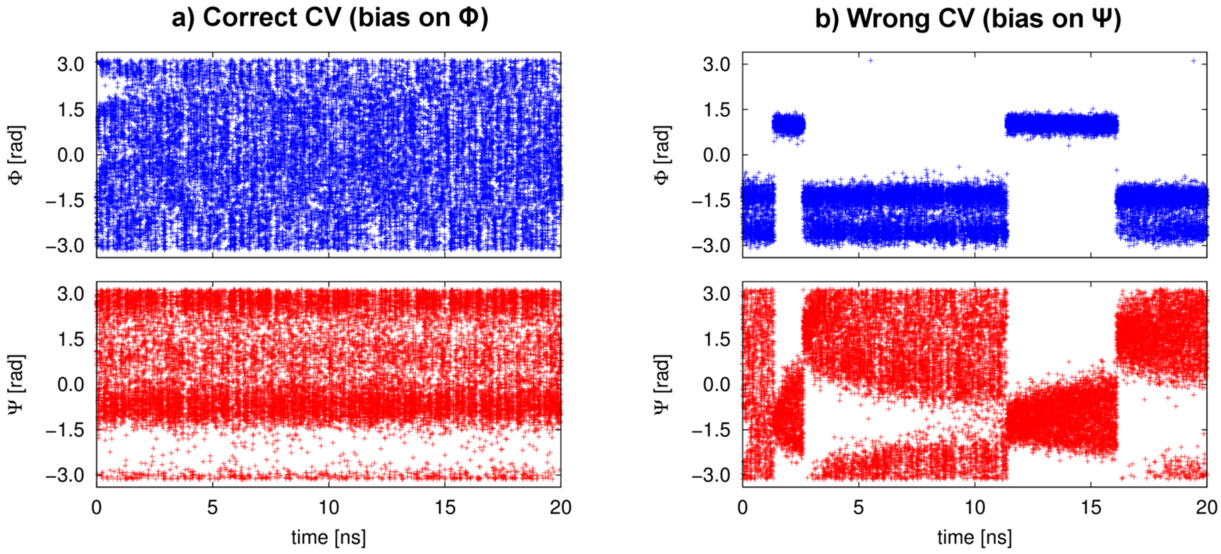


FIG. S5. Time evolution of the $\Phi$ and $\Psi$ during an optimization process for alanine dipeptide in vacuum at 300 K using either **a)** $\Phi$ or **b)** $\Psi$ as CV. The bias potential is expanded using 12 basis functions

SM for arXiv:1407.0477v3

### C. Localizing the Sampling of the CVs

As discussed above, we can use the flexibility in choosing $p(\mathbf{s})$ in $\Omega[V]$ to localize the sampling of the CVs to a certain subspace of the phase space. For an example of this, we consider alanine dipeptide in vacuum using both $\Phi$ and $\Psi$ as CVs and localize the sampling around the free energy basin in the top left corner of the free energy surface (approximately located around $\Phi = -2.0, \Psi = 1.5$) that is both more spread out and deeper in free energy and also has more structure than the other basin.

In order to properly account for the periodicity of CVs we use a Von Mises distribution for $p(\Phi, \Psi)$ and only consider the case where $\Phi$ and $\Psi$ are independent such that it can be written as a product of two one-dimensional Von Mises distributions

$$p(\Phi, \Psi) = p(\Phi) \cdot p(\Psi) = \frac{e^{\kappa_\Phi \cos(\Phi - \mu_\Phi)}}{2\pi I_0(\kappa_\Phi)} \cdot \frac{e^{\kappa_\Psi \cos(\Psi - \mu_\Psi)}}{2\pi I_0(\kappa_\Psi)}, \tag{S20}$$

where $I_0$ is a modified Bessel function of order 0 and the parameters $\mu$ and $\sqrt{1/\kappa}$ are comparable to the mean $\mu$ and standard deviation $\sigma$ of the normal distribution. We use the parameters $\mu_\Phi = -2.0$, $\mu_\Psi = 1.5$, and $\sqrt{1/\kappa_\Phi} = \sqrt{1/\kappa_\Psi} = 0.5$ in the calculation that results in the $p(\Phi, \Psi)$ shown in Fig. S6**a)**

As observed in Fig. S6**b)**, the sampling of $\Phi$ and $\Psi$ during the simulation is completely confined to the region around $\Phi = -2.0$ and $\Psi = 1.5$, respectively. Furthermore, the sampled distributions of $\Phi$ and $\Psi$ in Figs. S6**c)** and S6**d)** are in very good agreement with the targeted $p(\Phi, \Psi) = p(\Phi) \cdot p(\Psi)$.

We can then estimate the free energy surface by using the relation $F(\Phi, \Psi) = -V(\Phi, \Psi) - \frac{1}{\beta} \log p(\Phi, \Psi)$. Of course, this estimate will only be valid for the region that was sampled so we only get information about the free energy basin around $\Phi = -2.0, \Psi = 1.5$. For this basin the obtained $F(\Phi, \Psi)$ in Fig. S6**e)** is in excellent agreement with results in Fig. S2 above.

SM for arXiv:1407.0477v3

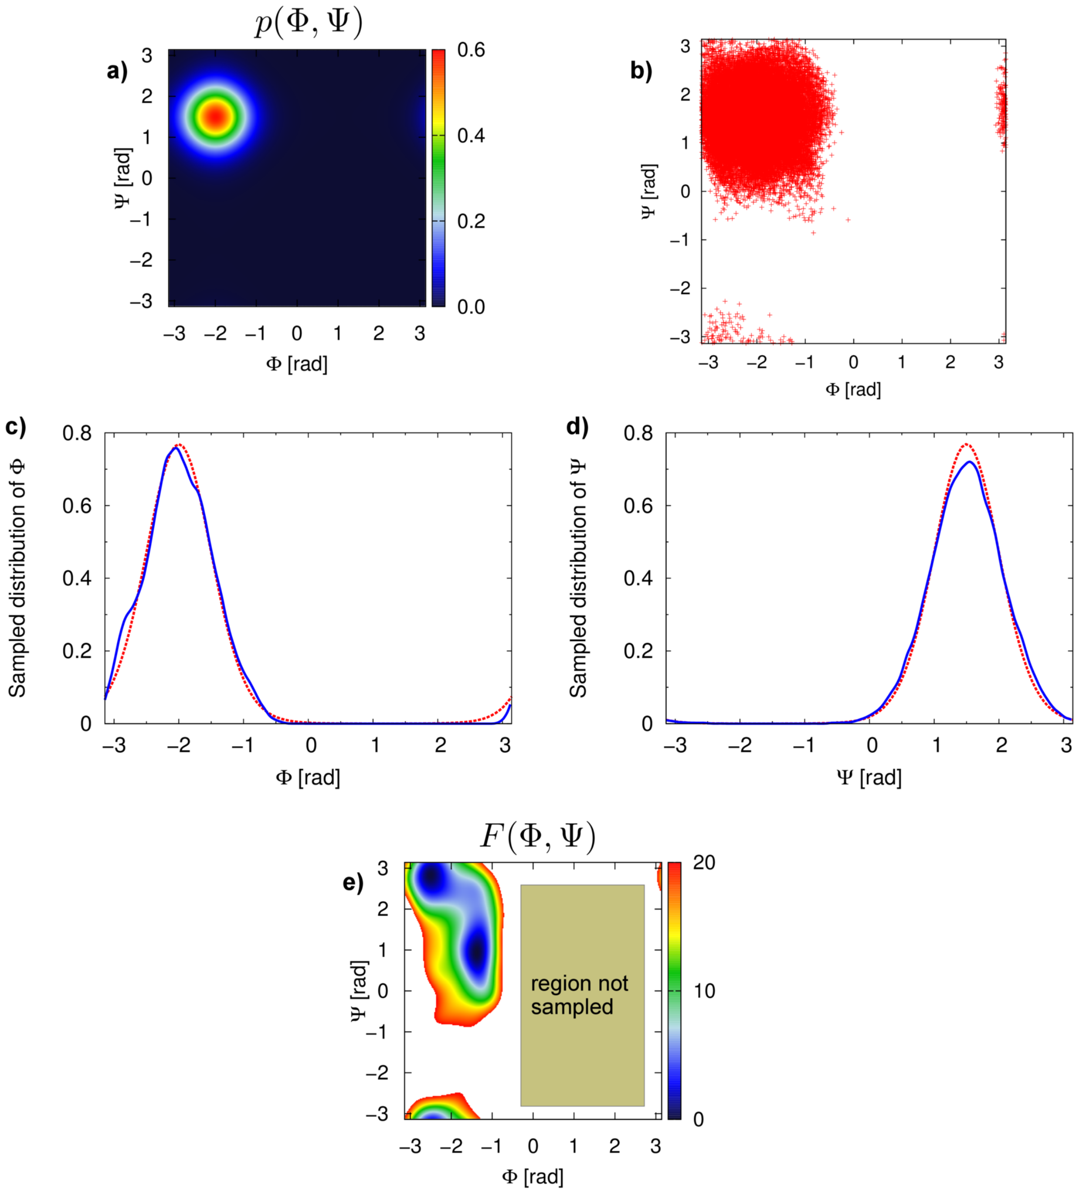


FIG. S6. Results obtained using the variational approach for alanine dipeptide in vacuum at 300 K where the sampling was localized around the free energy basin at $\Phi = -2.0, \Psi = 1.5$ as described in the text.

**a)** The Von Mises distribution $p(\Phi, \Psi)$ used to localize the sampling. **b)** The values in the $\Phi - \Psi$ plane sampled during the simulation. **c)** The sampled distribution of $\Phi$ (blue solid lines) from the simulation obtained using a kernel density estimation (Gaussian kernels with bandwidth of 0.05 rad). For comparison we also show the targeted Von Mises distribution $p(\Phi)$ (red dashed line). **d)** The sampled distribution of $\Psi$ (blue solid lines) from the simulation obtained using a kernel density estimation (Gaussian kernels with bandwidth of 0.05 rad). For comparison we also show the targeted Von Mises distribution $p(\Psi)$ (red dashed line). **e)** The FES $F(\Phi, \Psi)$ obtained from the simulation. The bias potential $V(\Phi, \Psi)$ is expanded using 13 basis functions per CV and the simulation is run for 10 ns.

SM for arXiv:1407.0477v3

### D. Variational Calculations for General CVs

As discussed in Section II the Fourier expansion of $V(\mathbf{s})$ can also be used for general non-periodic CVs by taking the domains of the CVs to larger than the range of CV values one is interested in. As an example of this we consider a two-dimensional, seven-particle, Lennard-Jones cluster that has previously been used as a benchmark system for reconnaissance metadynamics [10]. The free energy surface of this system can be described in terms of the second and third moments, $\mu_2^2$ and $\mu_3^3$, of the distribution of coordination numbers.

The bias potential $V(\mu_2^2, \mu_3^3)$ is expanded in a Fourier series and we furthermore employ a Gaussian $p(\mu_2^2, \mu_3^3)$ to avoid unnecessary sampling at edges of the bias potential. Further details are given in the Computational Details section above.

The free energy surface $F(\mu_2^2, \mu_3^3)$ has rather sharp features so it probably not optimal to use a Fourier series to expand the bias potential. Despite this, the variational approach gives a pretty good representation of the free energy surface, as compared to reference results from well-tempered metadynamics.

This results give already a very encouraging prospect of using the variational approach for any general CVs. This will be explored further in future publications where we will also consider other basis sets that might more suitable for general CVs.

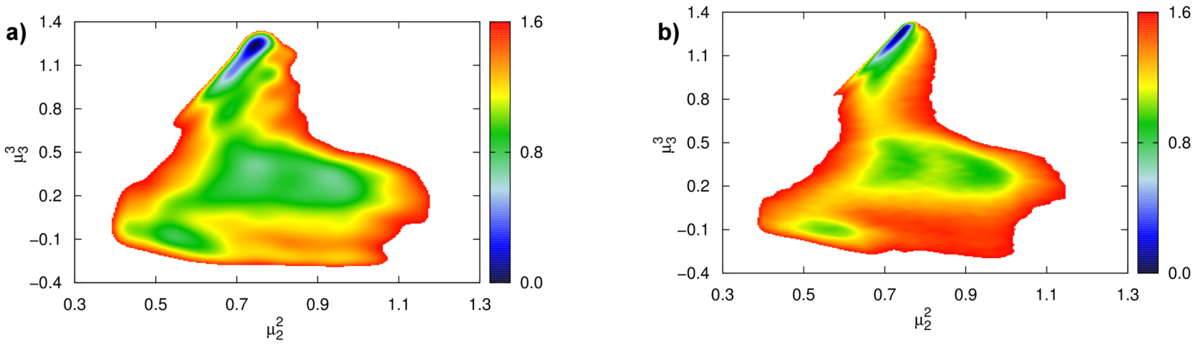


FIG. S7. The FES $F(\mu_2^2, \mu_3^3)$ for the two-dimensional, seven-particle, Lennard-Jones cluster at a temperature of $0.2\varepsilon$. **a)** FES $F(\mu_2^2, \mu_3^3)$ obtained with the variational approach. **b)** Reference results from well-tempered metadynamics simulation.

The color scale of the FES is given in Lennard-Jones units $\varepsilon$. All FES have their minimum value set to zero and are cut such that regions higher than 8 $k_{\mathrm{B}}T$ ($\approx 1.6\varepsilon$) are not shown.

SM for arXiv:1407.0477v3

### E. Further Free Energy Surfaces for $Ala_3$ in Vacuum

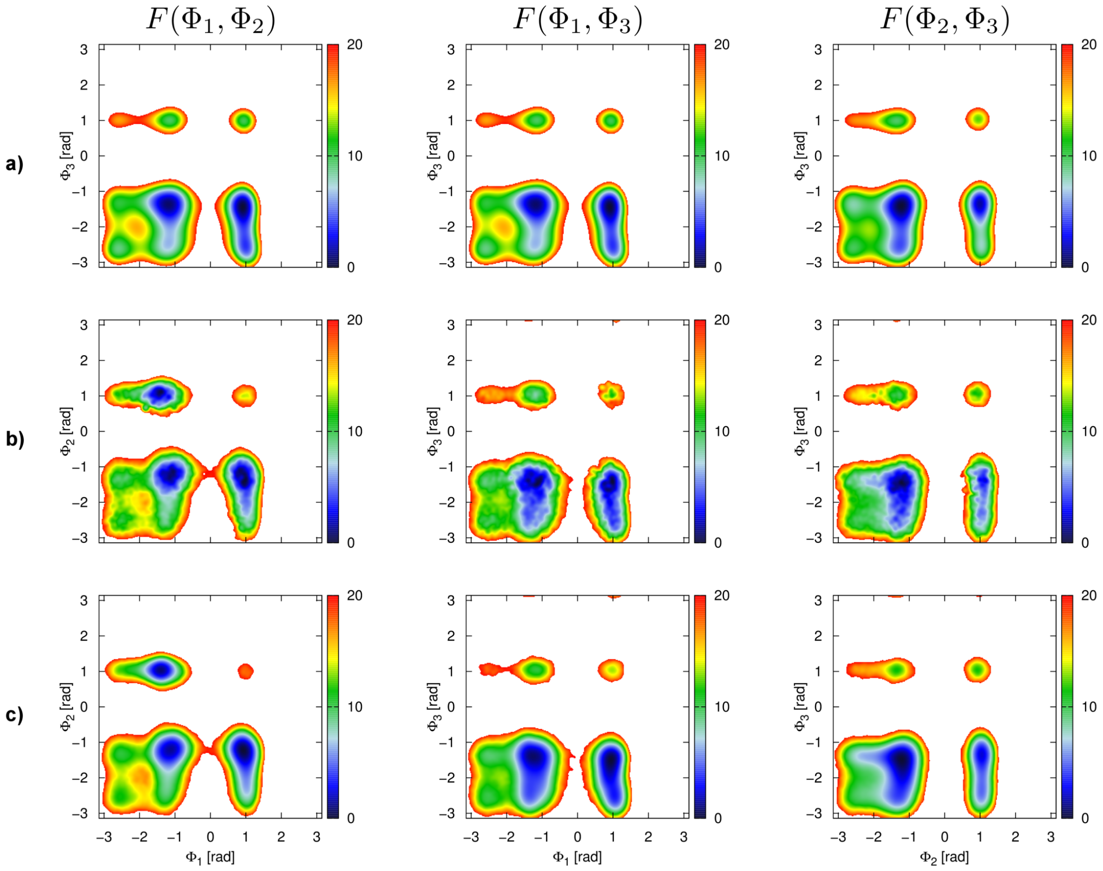


FIG. S8. Two-dimensional FES obtained with the variational approach for $Ala_3$ in vacuum at 300K using the backbone dihedral angles $\Phi_1$, $\Phi_2$, and $\Phi_3$ as CVs and 342 basis functions in the expansion of $V(\Phi_1, \Phi_2, \Phi_3)$.
For each FES we show: **a)** FES from a projection of $F(\Phi_1, \Phi_2, \Phi_3)$. **b)** FES obtained with on the fly reweighting. **c)** Reference results from a 500 ns parallel tempering simulation.
The color scale of the FES is given in units of kJ/mol. All FES have their minimum value set to zero and are cut such that regions higher than 8 $k_{\mathrm{B}}T$ ($\approx$ 20 kJ/mol) are not shown. The FES in **b)** and **c)** are obtained with kernel density estimation using a Gaussians kernel of bandwidth 0.05 rad for both CVs. The variational results are obtained after 100 ns of simulation time.

SM for arXiv:1407.0477v3

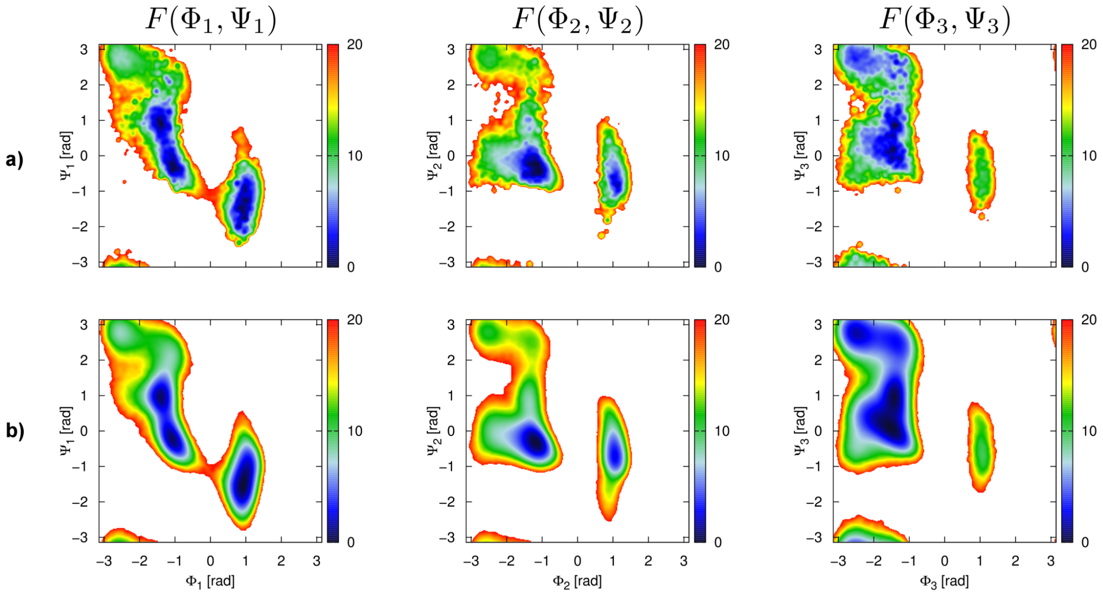


FIG. S9. Two-dimensional FES obtained with the variational approach for $Ala_3$ in vacuum at 300K using the backbone dihedral angles $\Phi_1$, $\Phi_2$, and $\Phi_3$ as CVs and 342 basis functions in the expansion of $V(\Phi_1, \Phi_2, \Phi_3)$.
For each FES we show: **a)** FES obtained with on the fly reweighting. **b)** Reference results from a 500 ns parallel tempering simulation.
The color scale of the FES is given in units of kJ/mol. All FES have their minimum value set to zero and are cut such that regions higher than 8 $k_{\mathrm{B}}T$ ($\approx$ 20 kJ/mol) are not shown. The FES in **a)** and **b)** are obtained with kernel density estimation using a Gaussians kernel of bandwidth 0.05 rad for both CVs. The variational results are obtained after 100 ns of simulation time.

SM for arXiv:1407.0477v3

[1] D. Branduardi, G. Bussi, and M. Parrinello, J. Chem. Theory Comput. **8**, 2247 (2012).

[2] V. Hornak, R. Abel, A. Okur, B. Strockbine, A. Roitberg, and C. Simmerling, Proteins: Structure, Function, and Bioinformatics **65**, 712 (2006).

[3] W. L. Jorgensen, J. Chandrasekhar, J. D. Madura, R. W. Impey, and M. L. Klein, J. Chem. Phys. **79**, 926 (1983).

[4] S. Pronk, S. Pall, R. Schulz, P. Larsson, P. Bjelkmar, R. Apostolov, M. R. Shirts, J. C. Smith, P. M. Kasson, D. van der Spoel, and et al., Bioinformatics **29**, 845 (2013).

[5] G. A. Tribello, M. Bonomi, D. Branduardi, C. Camilloni, and G. Bussi, Comput. Phys. Commun. **185**, 604 (2014).

[6] B. Hess, H. Bekker, H. J. C. Berendsen, and J. G. E. M. Fraaije, J. Comput. Chem. **18**, 1463 (1997).

[7] G. Bussi, D. Donadio, and M. Parrinello, J. Chem. Phys. **126**, 014101 (2007).

[8] U. Essmann, L. Perera, M. L. Berkowitz, T. Darden, H. Lee, and L. G. Pedersen, J. Chem. Phys. **103**, 8577 (1995).

[9] G. Bussi and M. Parrinello, Phys. Rev. E **75** (2007).

[10] G. A. Tribello, M. Ceriotti, and M. Parrinello, Proc. Natl. Acad. Sci. U.S.A. **107**, 17509 (2010).


SM for arXiv:1407.0477v3
